# Supplementary material for: Eliminating The Impossible, Whatever Remains Must Be True
Source: arXiv:2206.09551 source file (2022-11-30)
Supplement: Supplementary file 1 [file appendix.tex]

\newpage
\clearpage
\appendix
\appendixpage

\section{Proofs of Propositions}

\setcounter{proposition}{1}
\setcounter{remark}{0}

\begin{proposition}%[\cite{rubin-aaai22}]
	%
	% Let $\mbf{v}\in\mbb{F}$ be an instance such that
	% $\tau(\mbf{v})=c$, $c\in\fml{K}$.
	Consider $\mbf{v}\in\mbb{F}$ such that $\tau(\mbf{v})=c$,
	$c\in\fml{K}$, and background knowledge $\varphi$ is compatible with
	$\mbf{v}$.
	%
	% Assume that background knowledge $\varphi$ is compatible with all
	% the classes $c\in\fml{K}$, i.e.\ $\forall
	% (c\in\fml{K}).~\varphi(\mbf{x})\land\tau(\mbf{x})=c$ is
	% satisfiable.
	%
	Then for any subset-minimal AXp $\fml{X}\subseteq\fml{F}$ for
	prediction $\tau(\mbf{v})=c$, there is a subset-minimal AXp
	$\fml{X}'\subseteq\fml{F}$ for $\tau(\mbf{v})=c$ subject to
	background knowledge $\varphi$ such that $\fml{X}'\subseteq\fml{X}$.
	% \footnote{
	% 	The proofs of \textsc{Proposition 2} and \textsc{Proposition 3} are provided in the Appendix.
	% }
	%
\end{proposition}

\begin{proof}%[Sketch]
	First, observe that if~\eqref{eq:axp} holds for a set $\fml{S}$
	then~\eqref{eq:axpc} holds for $\fml{S}$ too.
	%
	% $\boxra$\;
	%
	Let $\fml{X}$ be a subset-minimal AXp for $\tau(\mbf{v})=c$ with no
	knowledge of $\varphi$, i.e.~\eqref{eq:axp} holds for $\fml{X}$.
	Thanks to the observation above,~\eqref{eq:axpc} also holds for
	$\fml{X}$.
	To make it subset-minimal subject to $\varphi$, we can apply linear
	search feature traversal (similar to the AXp extraction
	algorithm~\cite{inms-aaai19}) checking if any of the features of
	$\fml{X}$ can be dropped s.t.~\eqref{eq:axpc} still holds.
	The result subset-minimal set of features $\fml{X}'$ is the target
	AXp subject to knowledge $\varphi$.
\end{proof}

\begin{remark}
	Note that the opposite, i.e.\ that given AXp $\fml{X}'$ subject to
	background knowledge $\varphi$, there must exist a subset-minimal AXp
	$\fml{X}\supseteq\fml{X}'$ without background knowledge $\varphi$,
	in general does not hold.
	To illustrate a counterexample, consider a fully Boolean classifier
	$\tau:\{0,1\}^3\rightarrow\{0,1\}$ on features $\fml{F}=\{a, b,
	c\}$, which returns 1 iff $(a+b+c)\geq 2$.
	Consider instance $\mbf{v}=(1,1,0)$ classified as 1.
	Given knowledge $\varphi=(\neg{c}\rightarrow
	a)\land(\neg{c}\rightarrow b)$, a valid subset-minimal AXp is
	$\fml{X}'=\{c\}$.
	However, when discarding knowledge $\varphi$, the only
	subset-minimal AXp for $\mbf{v}$ is
	$\fml{X}=\{a,b\}\not\supseteq\fml{X}'$.
\end{remark}

\begin{proposition}
	Consider $\mbf{v}\in\mbb{F}$ such that $\tau(\mbf{v})=c$,
	$c\in\fml{K}$, and background knowledge $\varphi$ is compatible with
	$\mbf{v}$.
	%
	% Assume that background knowledge $\varphi$ is compatible with
	% instance $\mbf{v}\in\mbb{F}$.
	%
	% all the classes $c\in\fml{K}$, i.e.\ $\forall
	% (c\in\fml{K}).~\varphi(\mbf{x})\land\tau(\mbf{x})=c$ is
	% satisfiable.
	%
	Then for any subset-minimal CXp $\fml{Y}'\subseteq\fml{F}$ for
	prediction $\tau(\mbf{v})=c$ subject to knowledge
	$\varphi$, there is subset-minimal CXp $\fml{Y}\subseteq\fml{F}$ is
	a CXp for prediction $\tau(\mbf{v})=c$ such that
	$\fml{Y}'\supseteq\fml{Y}$.
\end{proposition}

\begin{proof}%[Sketch]
	First, observe that if~\eqref{eq:cxpc} holds for a set $\fml{S}$
	then~\eqref{eq:cxp} holds for $\fml{S}$ too.
	%
	%$\boxra$\;
	%%
	%Let $\fml{Y}$ be a subset-minimal CXp for $\tau(\mbf{v})=c$ with no
	%knowledge of $\varphi$, i.e.~\eqref{eq:cxp} holds for $\fml{Y}$.
	%%
	%Also let $\fml{Y}''=\fml{F} \supseteq \fml{Y}$.
	%%
	%Clearly,~\eqref{eq:cxpc} holds for $\fml{Y}''$ as there must be an
	%instance $\mbf{x}\in\mbb{F}$ compatible with $\varphi$ such that
	%$\tau(\mbf{x})\neq c$.
	%%
				%Now either $\fml{Y''}$ is subset-minimal Let us drop features
	%from $\fml{Y}''$ one-by-one testing the features of $\fml{Y}$ last.
	%%
	%Denote the result set $\fml{Y}'$.
	%%
	%By construction, either of the two holds:
	%(a)~$\fml{Y}'\subset\fml{Y}$ or (b)~$\fml{Y}'\supseteq\fml{Y}$.
	%%
	%However, the observation made at the beginning and
	%subset-minimality of $\fml{Y}$ exclude~(a).
	%
	% $\boxla$\;
	%
	Let $\fml{Y}'$ be a subset-minimal CXp subject to background
	knowledge $\varphi$, i.e.~\eqref{eq:cxpc} holds for $\fml{Y}'$.
	By the observation made above,~\eqref{eq:cxp} also holds for
	$\fml{Y}'$.
	Now, by applying linear search dropping features of $\fml{Y}'$ and
	checking~\eqref{eq:cxp}~\cite{inms-aaai19}, one can get a
	subset-minimal $\fml{Y}\subseteq\fml{Y}'$ wrt.~\eqref{eq:cxp}, i.e.\
	$\fml{Y}$ is a subset-minimal CXp.
\end{proof}

\begin{remark}
	Note that the reverse direction: given a CXp $\fml{Y}$ generated
	without using background knowledge, there must exists a CXp
	$\fml{Y'} \supseteq \fml{Y}$ using background knowledge, does not
	hold.
	Consider a classifier on Boolean features $\fml{F} = \{a,b,c\}$
	which returns the parity ODD, EVEN of $a+b+c$.
	Consider background knowledge $a = b$.
	Now $\fml{Y} = \{a\}$ is a CXp for $\tau(1,1,1)=\text{ODD}$ without
	using background knowledge supported by instance
	$\tau(0,1,1)=\text{EVEN}$.
	But this does not agree with the background knowledge.
	The only CXp using the background knowledge is $\{c\}$, because $a$
	and $b$ must change together they never affect the parity.
	However and as our experimental results confirm, in practice these
	examples do not arise, as we always find a CXp using
	background knowledge that extends a CXp without background
	knowledge.
\end{remark}

% \newpage
% \section{Pseudo-codes}
% \begin{algorithm}[h!]
% 	\caption{Determine Background Knowledge Used}\label{alg:usedrules}
% 	\textbf{Input}: Classifier $\tau$, instance $\mbf{v}$, prediction $c=\tau(\mbf{v})$,
% 		constraints $\varphi$, AXp $\fml{X}'$ \\
% 	\textbf{Output} Used rules: $\varphi_u\subseteq\varphi$
% 	\begin{algorithmic}[1]
% 		\STATE $\varphi_u \gets \varphi$
% 		\IF {\label{ln:check1}$\texttt{Entails}(\fml{X}', \tau, \mbf{v}, c, \emptyset$)}
% 		\RETURN $\emptyset$
% 		\ENDIF
% 		\FOR {$r \in \varphi$}
% 			\IF {\label{ln:check2}$\texttt{Entails}(\fml{X}', \tau, \mbf{v}, c, \varphi_u \setminus \{r\}$)}
% 			\STATE $\varphi_u  \gets \varphi_u  \setminus \{r\}$
% 			\ENDIF
% 		\ENDFOR
% 		\RETURN $\varphi_u$
% 	\end{algorithmic}
% \end{algorithm}

\newpage
\section{Rule Extraction with xcon}
\begin{figure}[!ht]
  \centering
  % \begin{subfigure}[b]{0.46\textwidth}
    \centering
    \includegraphics[width=0.46\textwidth]{avg_accry}
    \caption{Accuracy of rules extracted by \emph{xcon}.}
    \label{fig:raccry}
\end{figure}

Additionally to Table~\ref{tab:racry}, Figure~\ref{fig:raccry} details
the average accuracy of the background knowledge extracted, including
the rules of all the aforementioned sizes
($rules_{all}$ represents all extracted rules while $rules_{1 \dots
5}$ indicates the extracted rules with corresponding size of $1$ to
$5$).
As can be observed, average rule accuracy gets no lower than 94\%.
Furthermore, the average accuracy of \emph{all rules} in all datasets
is over 98\%.
Finally, for the majority of datasets, the accuracy of $rules_s$,
$s\in 1..5$, also exceeds 98\%.

\begin{figure*}[!ht]
	\begin{subfigure}[b]{0.244\textwidth}
    \centering
    \includegraphics[width=\textwidth]{bt/bt_exprtime_abd_scatter}
    \caption{AXp runtime for BTs}
    \label{fig:btaxprtime}
  \end{subfigure}
  \hfill
  \begin{subfigure}[b]{0.244\textwidth}
    \centering
    \includegraphics[width=\textwidth]{bt/bt_exprtime_con_scatter}
    \caption{CXp runtime for BTs}
    \label{fig:btcxprtime}
  \end{subfigure}
  \hfill
  \begin{subfigure}[b]{0.23\textwidth}
    \centering
    \includegraphics[width=\textwidth]{bt/bt_minsize_abd_scatter}
    \caption{AXp size for BTs}
    \label{fig:btaxp}
  \end{subfigure}%
  \hfill
  \begin{subfigure}[b]{0.23\textwidth}
    \centering
    \includegraphics[width=\textwidth]{bt/bt_minsize_con_scatter}
    \caption{CXp size for BTs}
    \label{fig:btcxp}
  \end{subfigure}
  \caption{Impact of \emph{xcon} rules on runtime~(ms) and explanation size for BTs.}
  \label{fig:btxprtime}
\end{figure*}

\begin{figure*}[!ht]
	\begin{subfigure}[b]{0.244\textwidth}
    \centering

    \includegraphics[width=\textwidth]{bnn/bnn_exprtime_abd_scatter}
    \caption{AXp runtime for BNNs}
    \label{fig:bnnaxprtime}
  \end{subfigure}
  \hfill
  \begin{subfigure}[b]{0.244\textwidth}
    \centering
    \includegraphics[width=\textwidth]{bnn/bnn_exprtime_con_scatter}
    \caption{CXp runtime for BNNs}
    \label{fig:bnncxprtime}
  \end{subfigure}
  \hfill
  \begin{subfigure}[b]{0.23\textwidth}
    \centering
    \includegraphics[width=\textwidth]{bnn/bnn_minsize_abd_scatter}
    \caption{AXp size for BNNs}
    \label{fig:bnnaxp}
  \end{subfigure}%
  \hfill
  \begin{subfigure}[b]{0.23\textwidth}
    \centering
    \includegraphics[width=\textwidth]{bnn/bnn_minsize_con_scatter}
    \caption{CXp size for BNNs}
    \label{fig:bnncxp}
  \end{subfigure}
  \caption{Impact of \emph{xcon} rules on runtime~(ms) and explanation size for BNNs.}
  \label{fig:bnnxprtime}
\end{figure*}

\newpage
\section{Knowledge-Assisted Explanations for BTs and BNNs with xcon}

The scatter plots in Figures~\ref{fig:btxprtime}
and~\ref{fig:bnnxprtime} overview the results for AXp and CXP runtime
as well as AXp and CXp size for BTs and BNNs, respectively.
While there is no significant trend in the runtime, explanation size
changes similarly to the case of DL models discussed in the paper.
In particular, in many cases the size of a smallest AXp drops from 11
to 2, and from 17 to 2, for BTs, and BNNs, respectively.
%
%\autoref{fig:dlaxp} shows that the size of smallest AXps can
%dramatically drop from $14$ to $2$ in DLs when background knowledge
%is applied.
%%
%A similar observation can be made wrt.~BT and BNN models, where the
%size of AXps drops from 13 to 2 and from 17 to 2, respectively.
%
% while the size can significantly decrease from $13$ to $2$ in
% BTs~(see \autoref{fig:btaxp}).
%
% The size of the smallest AXp can fall from $17$ to $2$ in BNNs in
% \autoref{fig:bnnaxp}).
%
In contrast to AXps, Figures~\ref{fig:btcxp} and \ref{fig:bnncxp}
illustrate that the size of smallest CXps is increased when background
knowledge is applied.
Namely, in a number of cases the size of a smallest CXp jumps from 1
to 15, and from 2 to 13 for BTs, and BNNs, respectively.
% The size of smallest CXps can jump considerably from $2$ to $13$ in
% DLs, BTs and BNNs.
%
These results exemplify how easy it is to flip the prediction when no
background knowledge is present illustrating the potential correctness
issues for the corresponding CXps.

A short summary of the changes in the explanation size is additionally
provided in Table~\ref{tab:exp} below where we selected 4 well-known
datasets widely studied in the context of explainability and
algorithmic fairness.

\begin{table}[h]
\centering
\caption{Change of average minimum explanation size.}
\label{tab:exp}
\scalebox{0.84}{
\begin{tabular}{ccccccc}\toprule
	\multirow{2}{*}{Dataset} & \multirow{2}{*}{Feats}  & \multirow{2}{*}{Model} & \multicolumn{2}{c}{AXp Size} &
	\multicolumn{2}{c}{CXp Size}  \\ \cmidrule{4-7}
				 & & & Before & After & Before & After  \\ \midrule
 &  & DL & 7.46 & 3.65 & 1.00 & 1.60 \\
adult & 65 & BT & 5.02 & 2.84 & 1.10 & 2.13 \\
 &  & BNN & 7.51 & 3.00 & 1.40 & 2.15 \\\midrule
 &  & DL & 5.65 & 3.74 & 1.01 & 1.15 \\
compas & 16 & BT & 3.91 & 3.09 & 1.06 & 1.15 \\
 &  & BNN & 4.40 & 2.79 & 1.19 & 1.30 \\\midrule
 &  & DL & 5.30 & 4.30 & 1.00 & 1.41 \\
lending & 35 & BT & 1.99 & 1.80 & 1.00 & 2.04 \\
 &  & BNN & 4.36 & 2.49 & 1.35 & 1.90 \\\midrule
 &  & DL & 9.51 & 5.58 & 1.00 & 1.23 \\
recidivism & 29 & BT & 6.04 & 4.04 & 1.17 & 1.67 \\
 &  & BNN & 7.01 & 4.01 & 1.42 & 1.82 \\\bottomrule
\end{tabular}
}
\end{table}

\newpage
\section{Rule Extraction with Apriori}
\begin{figure}[!ht]
	\centering
    \includegraphics[width=0.3\textwidth]{apriori/avg_5_rtime_scatter}
    \caption{Runtime between \emph{apriori} and \emph{xcon}.}
  \label{fig:aprirtime}
\end{figure}
Figure~\ref{fig:aprirtime} compares the runtime of rule extraction
between Apriori and the MaxSAT approach, where only rules of size up to $5$ are extracted by the
two approaches.
Note that Apriori only extracts rules of confidence~$100\%$ in the experiment,
such that all the rules extracted are
perfectly consistent with the \emph{known} data.
The average results across all $5$ train-test pairs were calculated.
Figure~\ref{fig:aprirtime} demonstrates that \emph{xcon} can extract rules
faster than Apriori in the vast majority of the considered datasets.
Moreover, Apriori can only extract rules in the all train-test
trunks of $57$~(out of $62$) datasets, while \emph{xcon}
is able to extract rules in all considered datasets.
As for the number of rules extracted by Apriori, for the datasets
solved it equals the number of rules extracted by Eclat and so the
reader is referred to Figure~\ref{fig:eclatsizenrules} for details.

%\paragraph{Rule Amount.} Figure~\ref{fig:aprisizenrules} depicts the comparison of the number of extracted rules
%in the $57$ datasets solved by both approaches. As can be observed, Apriori extracts more rules than \emph{xcon} since Apriori is unable to extract rules containing the negation of a feature value pair. For example,
%assume \emph{xcon} can extract a rule IF $x_1 \not = 0 $ THEN $x_2 = 1$, given feature~$1$, $2$ and their domains~$\fml{D}_1 = \fml{D}_2 = \{0, 1, 2\}$. However, Apriori can only extract two rules to represent the same information, i.e. IF $x_1 = 1 $ THEN $x_2 = 1$, and IF $x_1 = 2 $ THEN $x_2 = 1$.

\ignore{
\begin{figure*}[!ht]
	\centering
	%
%	\begin{subfigure}[b]{0.32\textwidth}
%    	\centering
%    	\includegraphics[width=\textwidth]{apriori/avg_all_rtime_scatter}
%    \caption{Comparison of runtime between $apriori_{all}$ and $xcon_{all}$}
%    \label{fig:apriallrtime}
%  \end{subfigure}
%  \hfill
  \begin{subfigure}[b]{0.37\textwidth}
    \centering
    \includegraphics[width=\textwidth]{apriori/avg_5_rtime_scatter}
    \caption{Runtime Comparison}
    \label{fig:aprisizertime}
  \end{subfigure}
  \begin{subfigure}[b]{0.36\textwidth}
    \centering
    \includegraphics[width=\textwidth]{apriori/avg_5_rules_scatter}
    \caption{Number of Rules Comparison}
    \label{fig:aprisizenrules}
  \end{subfigure}
    \caption{Runtime and number of rules comparison between \emph{apriori} and \emph{xcon}.}
  \label{fig:aprirtime}
\end{figure*}
}

\begin{figure*}[!ht]
	\centering
	\begin{subfigure}[b]{0.236\textwidth}
    \centering
    \includegraphics[width=\textwidth]{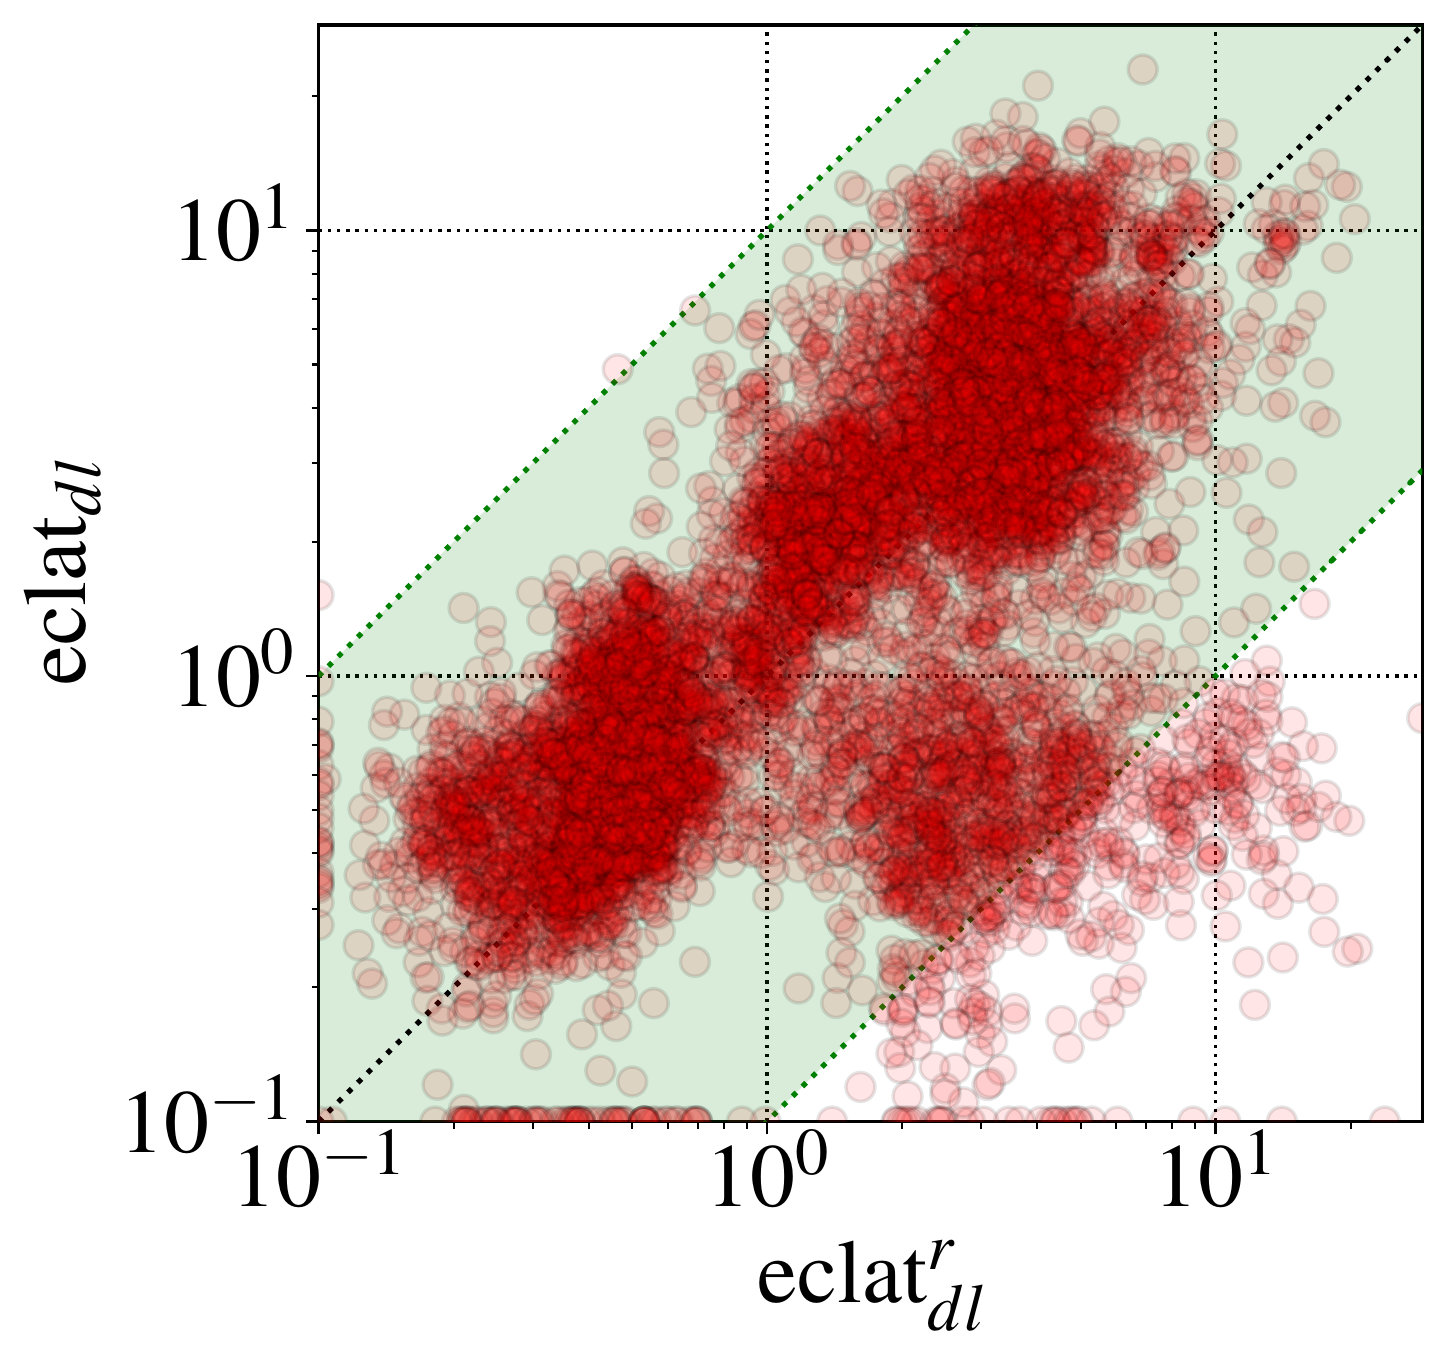}
    \caption{AXp runtime for DLs}
    \label{fig:adlaxprtime}
  \end{subfigure}
  \hfill
  \begin{subfigure}[b]{0.236\textwidth}
    \centering
    \includegraphics[width=\textwidth]{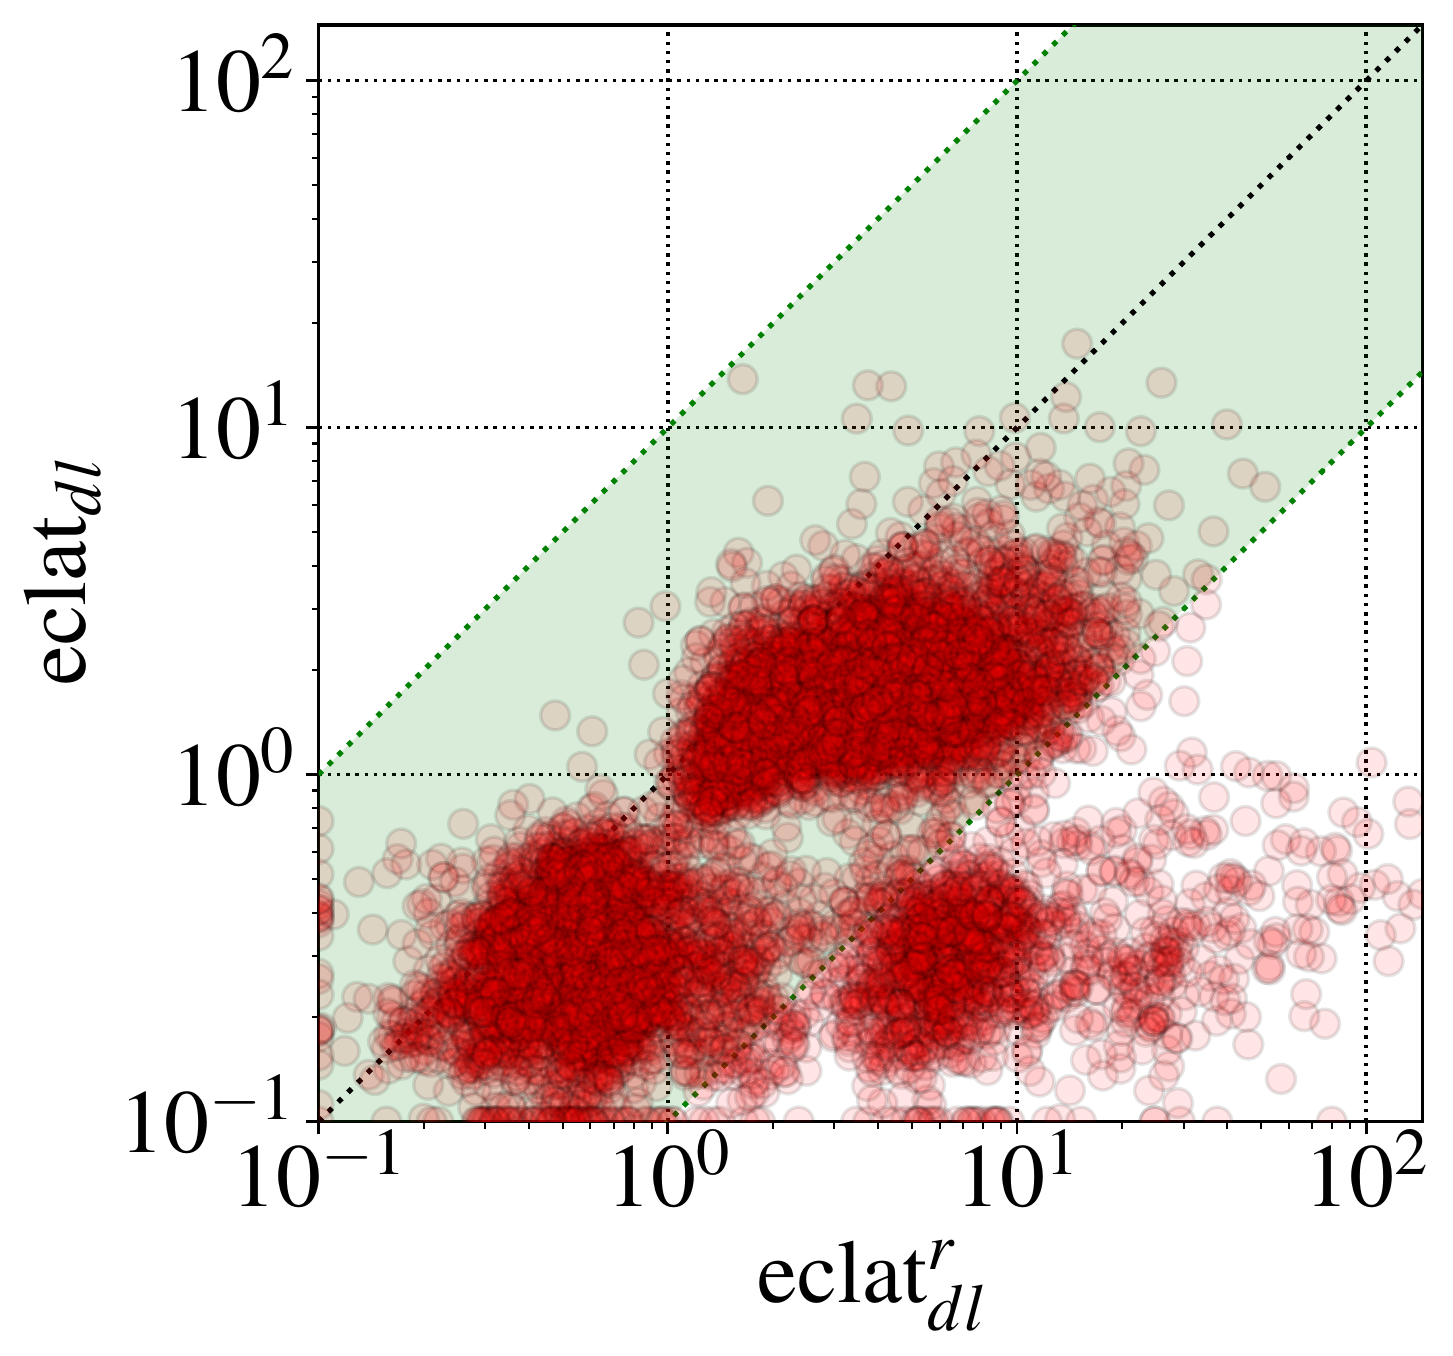}
    \caption{CXp runtime for DLs}
    \label{fig:adlcxprtime}
  \end{subfigure}
  \hfill
  \begin{subfigure}[b]{0.222\textwidth}
    \centering
    \includegraphics[width=\textwidth]{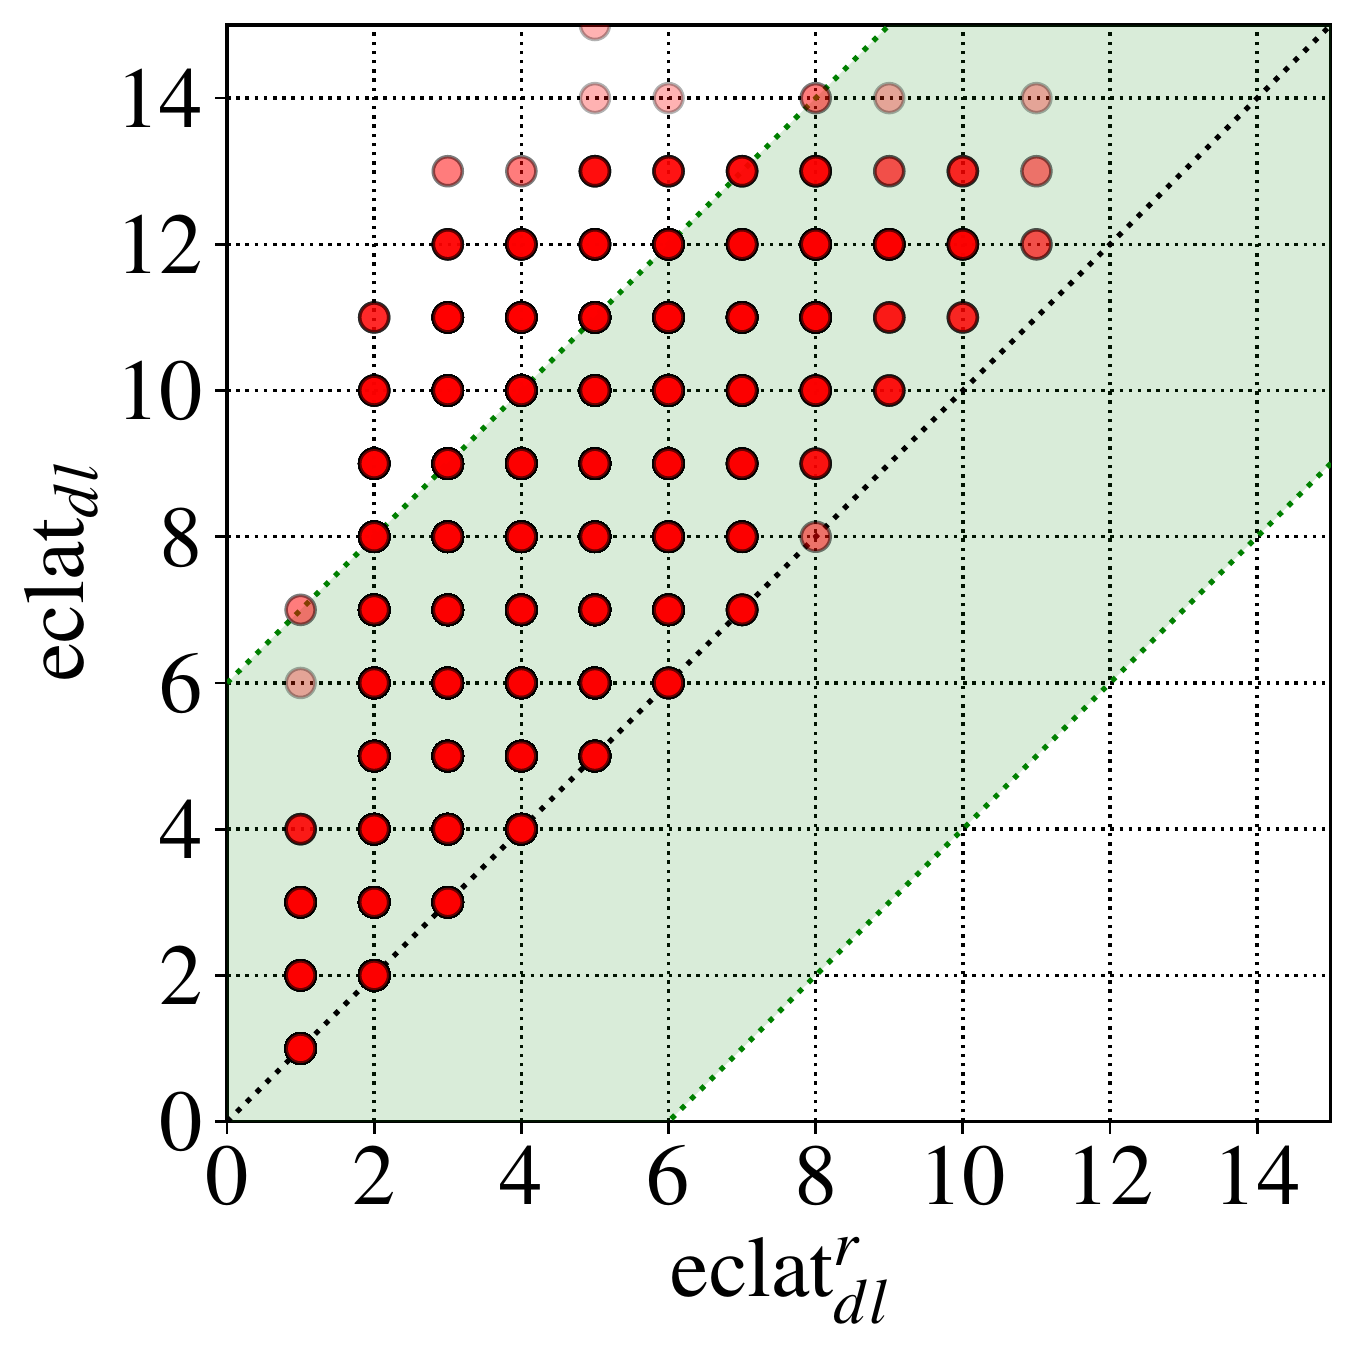}
    \caption{AXp size for DLs}
    \label{fig:adlaxp}
  \end{subfigure}%
  \hfill
  \begin{subfigure}[b]{0.222\textwidth}
    \centering
    \includegraphics[width=\textwidth]{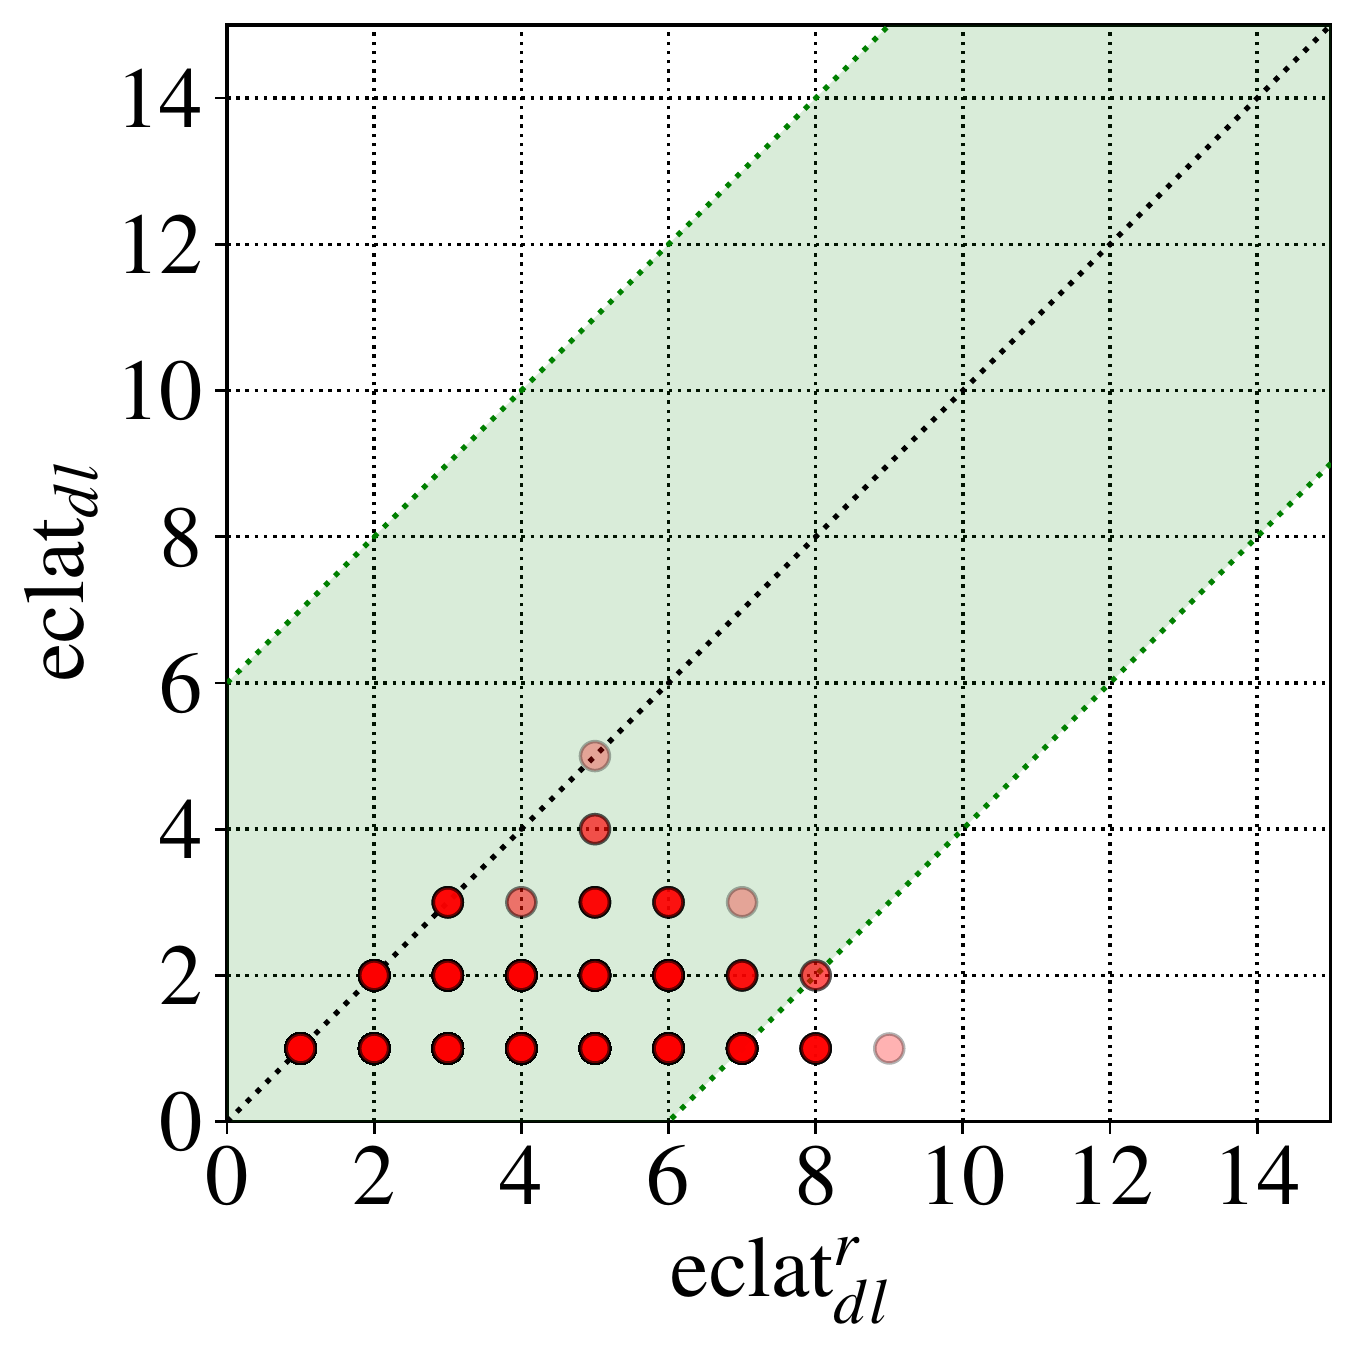}
    \caption{CXp size for DLs}
    \label{fig:adlcxp}
  \end{subfigure}
    \caption{Runtime~(ms) and explanation size for DLs w/wo Eclat-assisted background knowledge.}
  \label{fig:adlxp}
\end{figure*}

\begin{figure*}[!ht]
	\centering
	\begin{subfigure}[b]{0.236\textwidth}
    \centering
    \includegraphics[width=\textwidth]{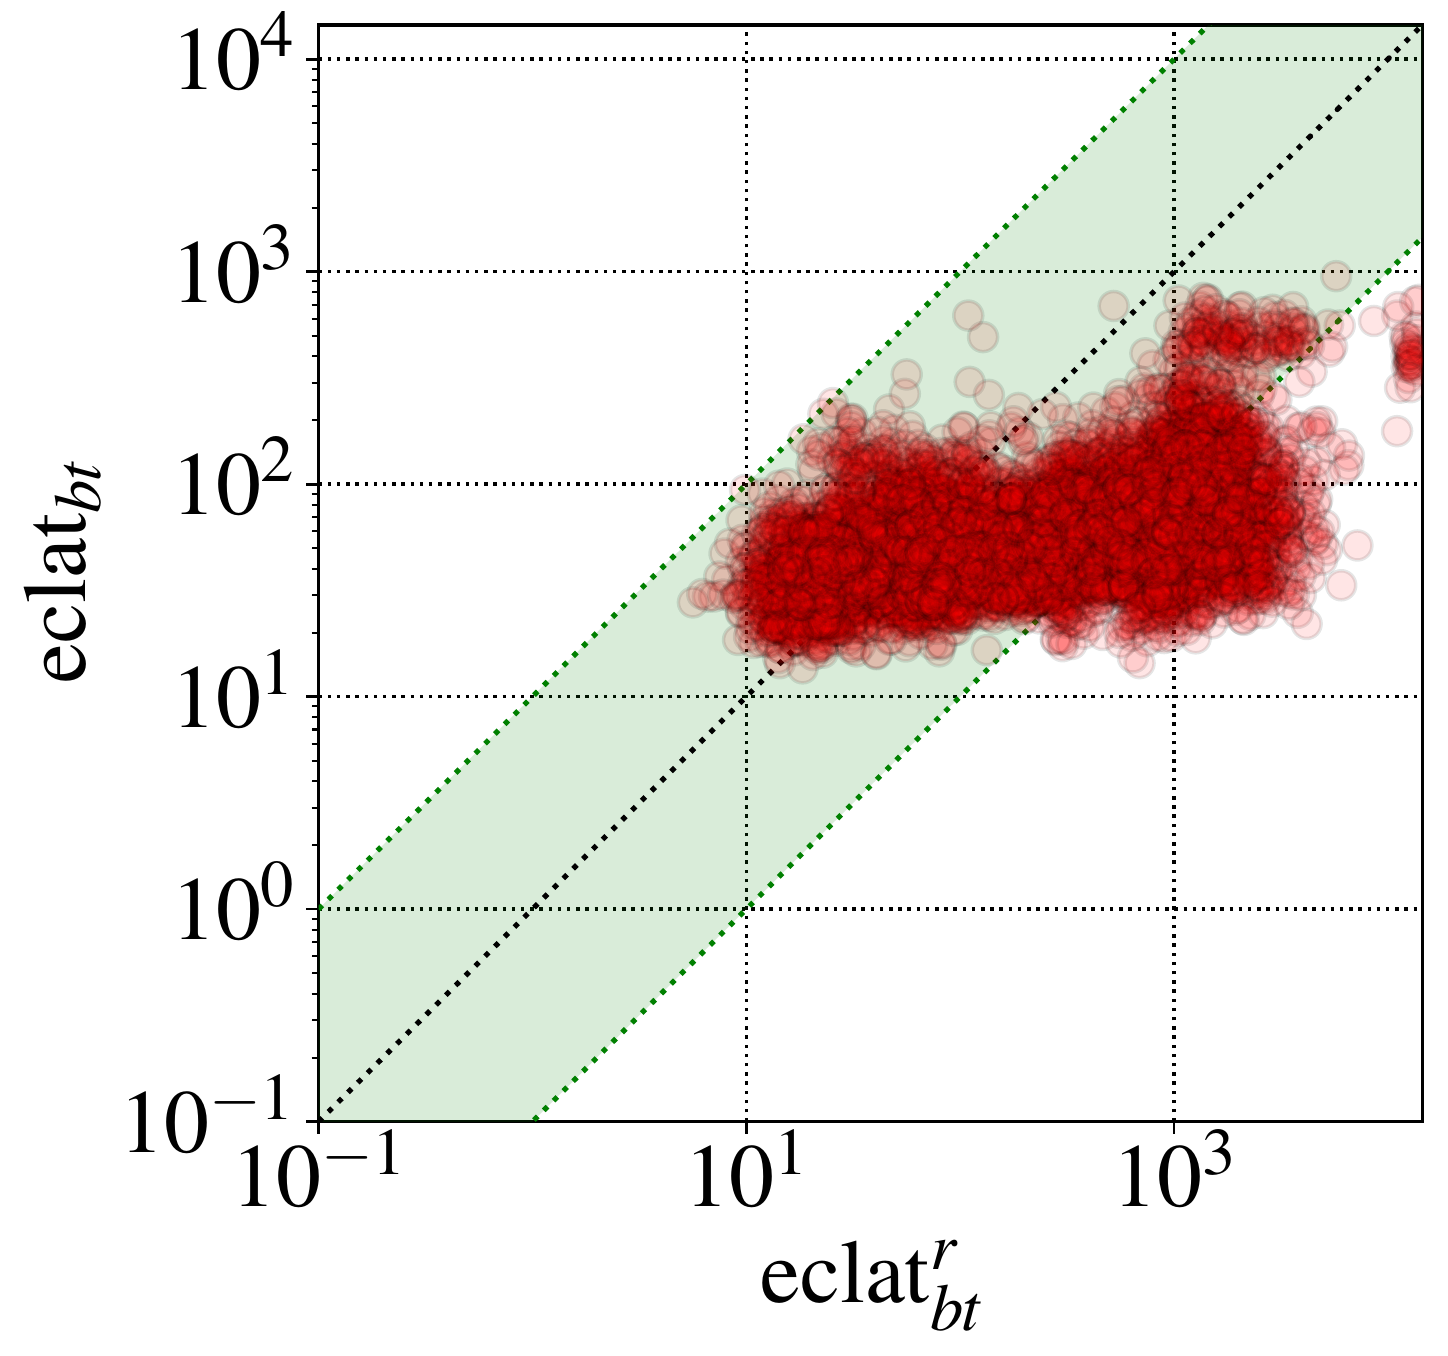}
    \caption{AXp runtime for BTs}
    \label{fig:abtaxprtime}
  \end{subfigure}
  \hfill
  \begin{subfigure}[b]{0.236\textwidth}
    \centering
    \includegraphics[width=\textwidth]{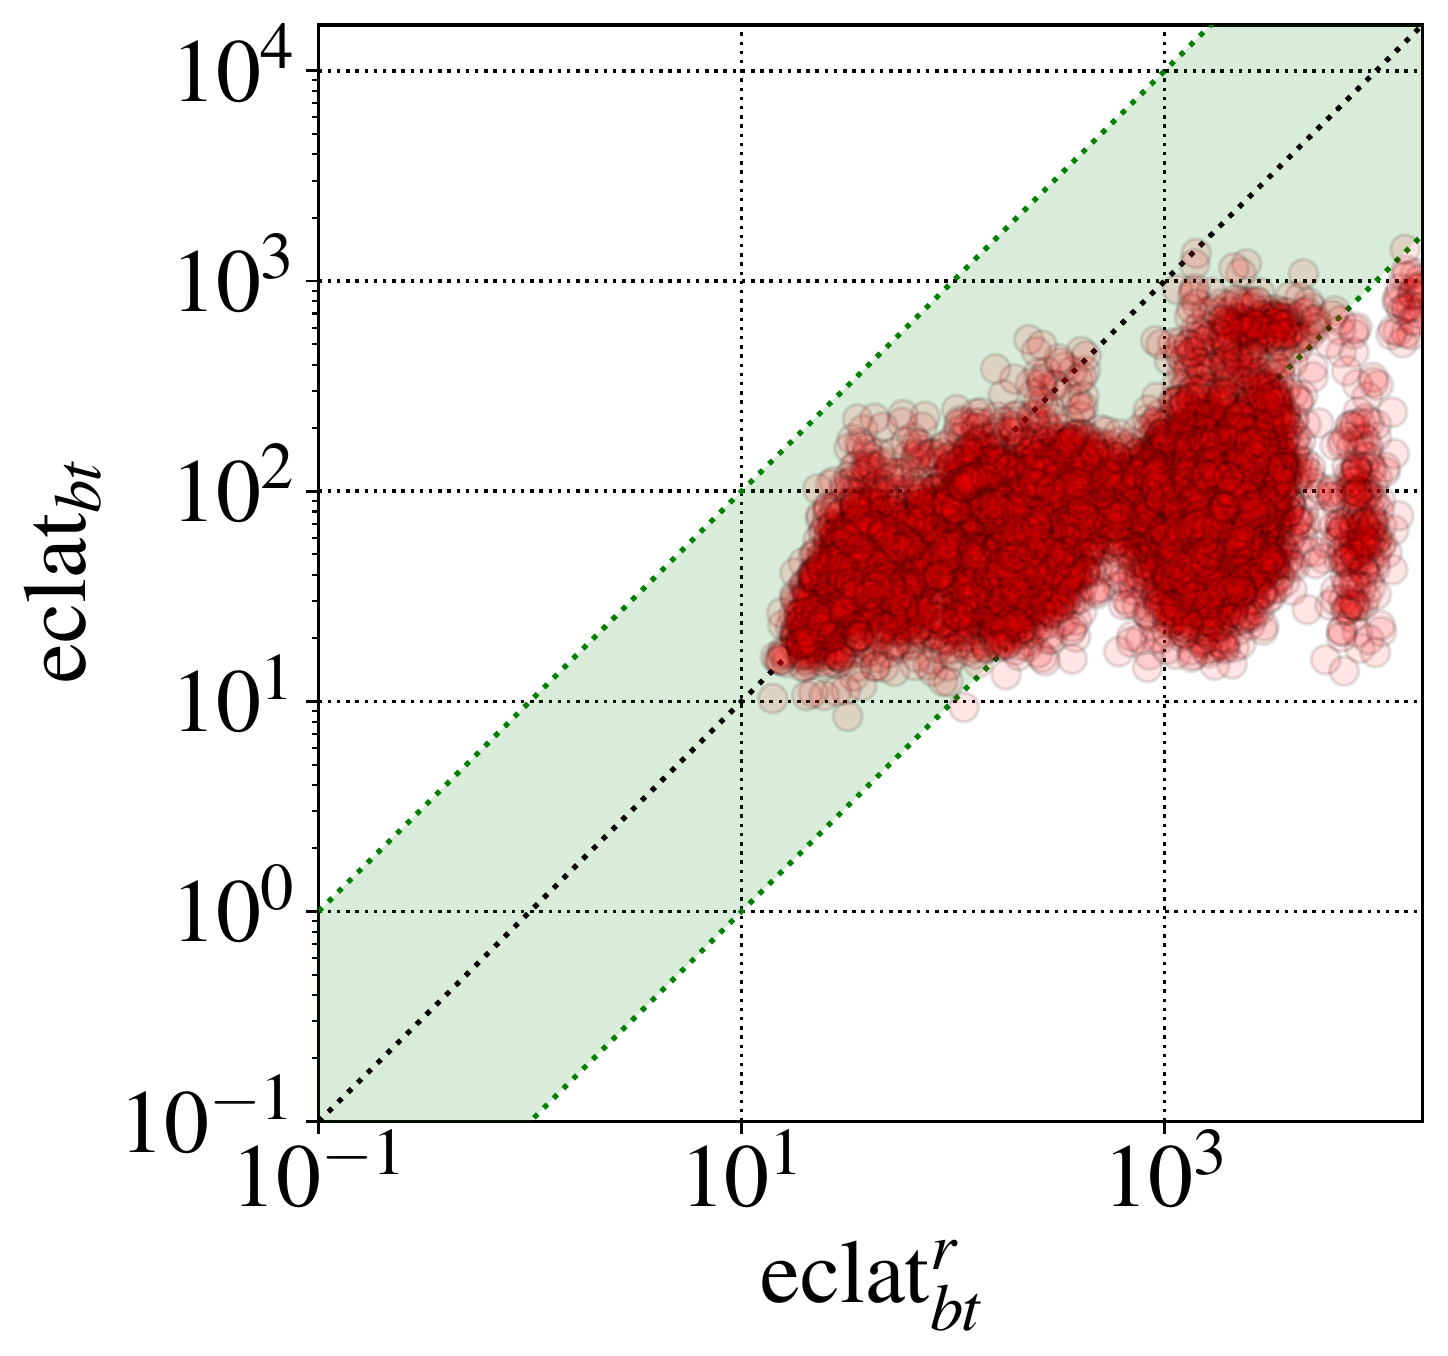}
    \caption{CXp runtime for BTs}
    \label{fig:abtcxprtime}
  \end{subfigure}
  \hfill
  \begin{subfigure}[b]{0.229\textwidth}
    \centering
    \includegraphics[width=\textwidth]{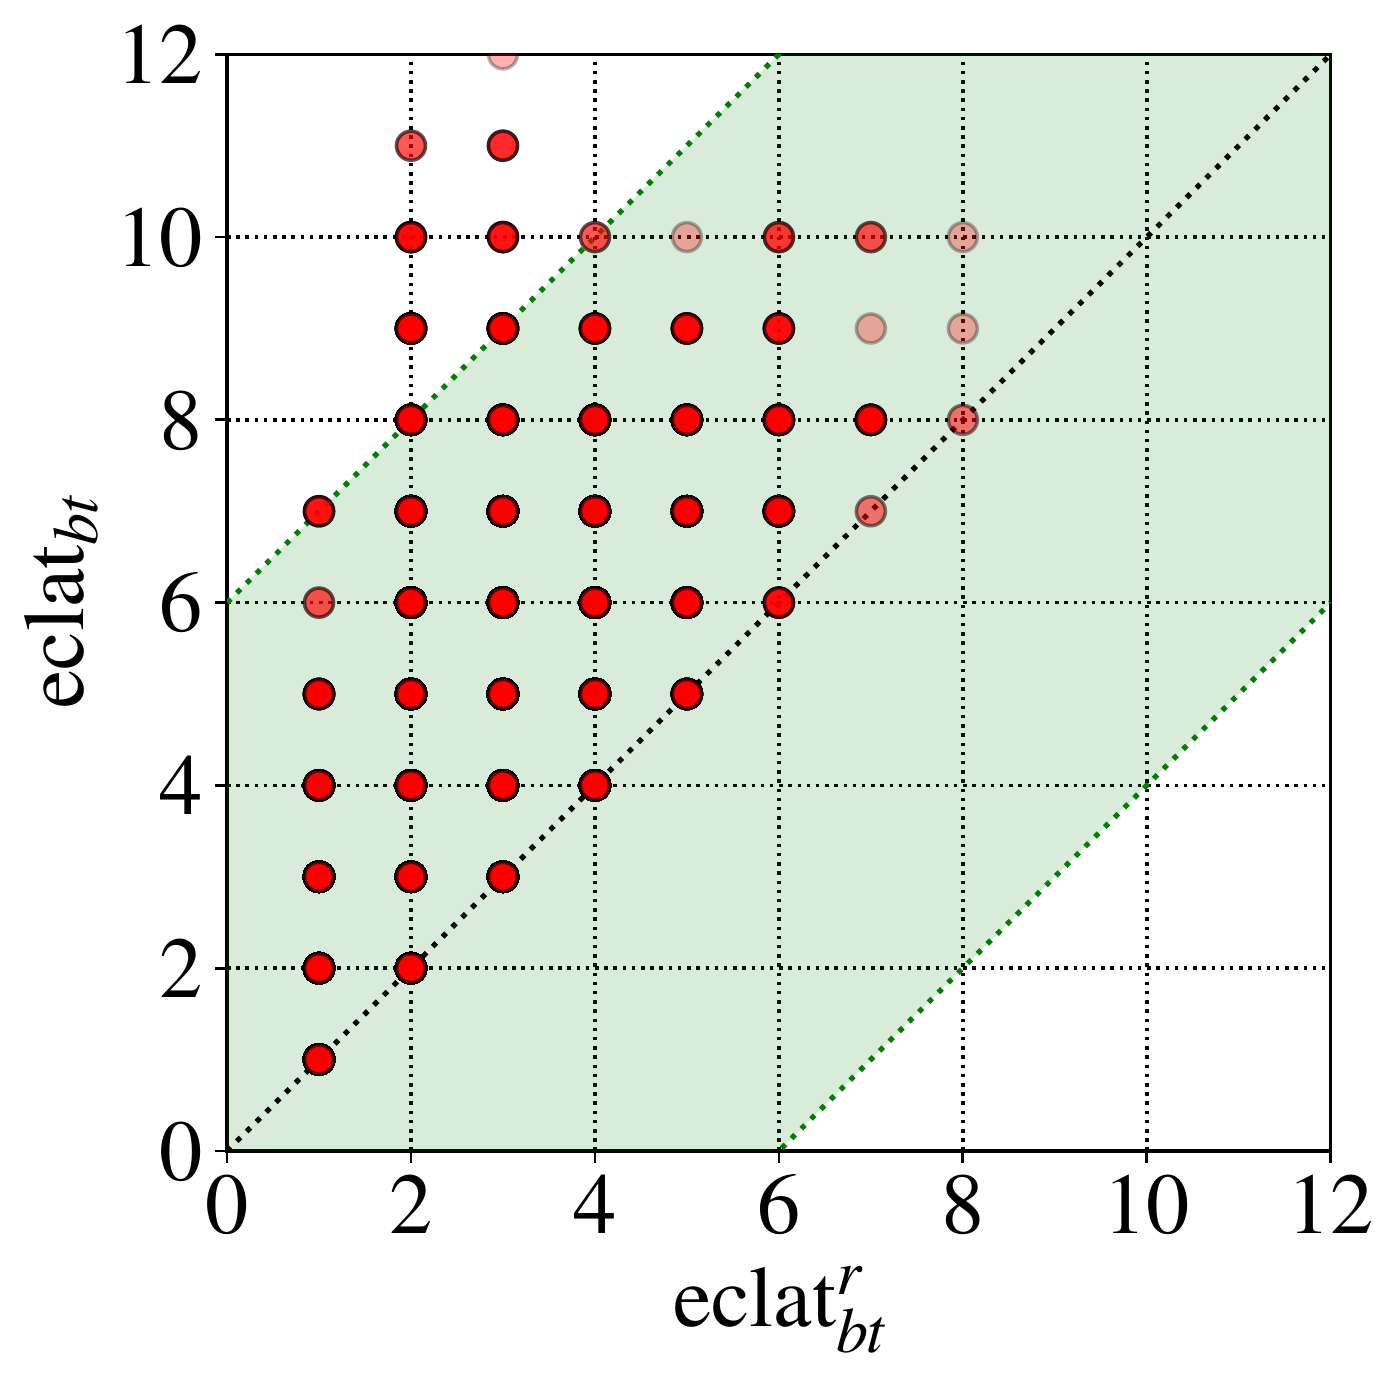}
    \caption{AXp size for BTs}
    \label{fig:abtaxp}
  \end{subfigure}%
  \hfill
  \begin{subfigure}[b]{0.229\textwidth}
    \centering
    \includegraphics[width=\textwidth]{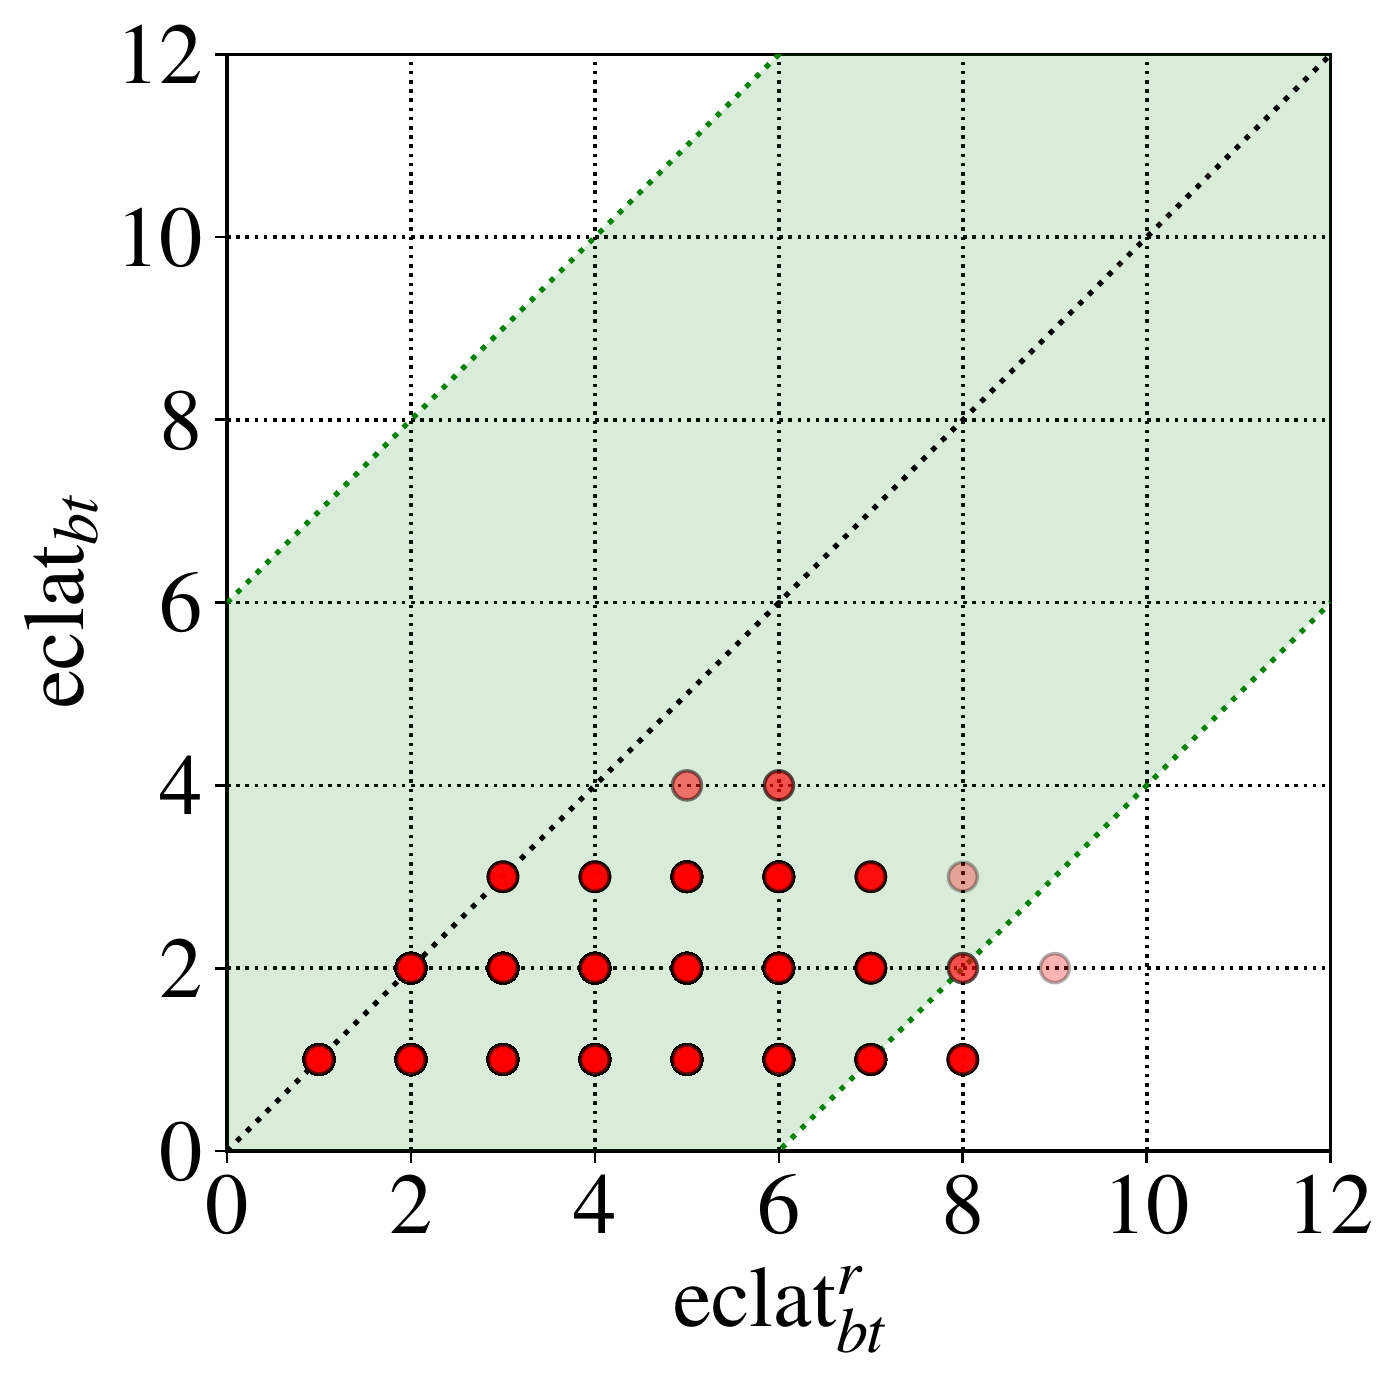}
    \caption{CXp size for BTs}
    \label{fig:abtcxp}
  \end{subfigure}
    \caption{Runtime~(ms) and explanation size for BTs w/wo Eclat-assisted background knowledge.}
  \label{fig:abtxp}
\end{figure*}

\begin{figure*}[!ht]
	\centering
	\begin{subfigure}[b]{0.236\textwidth}
    \centering
    \includegraphics[width=\textwidth]{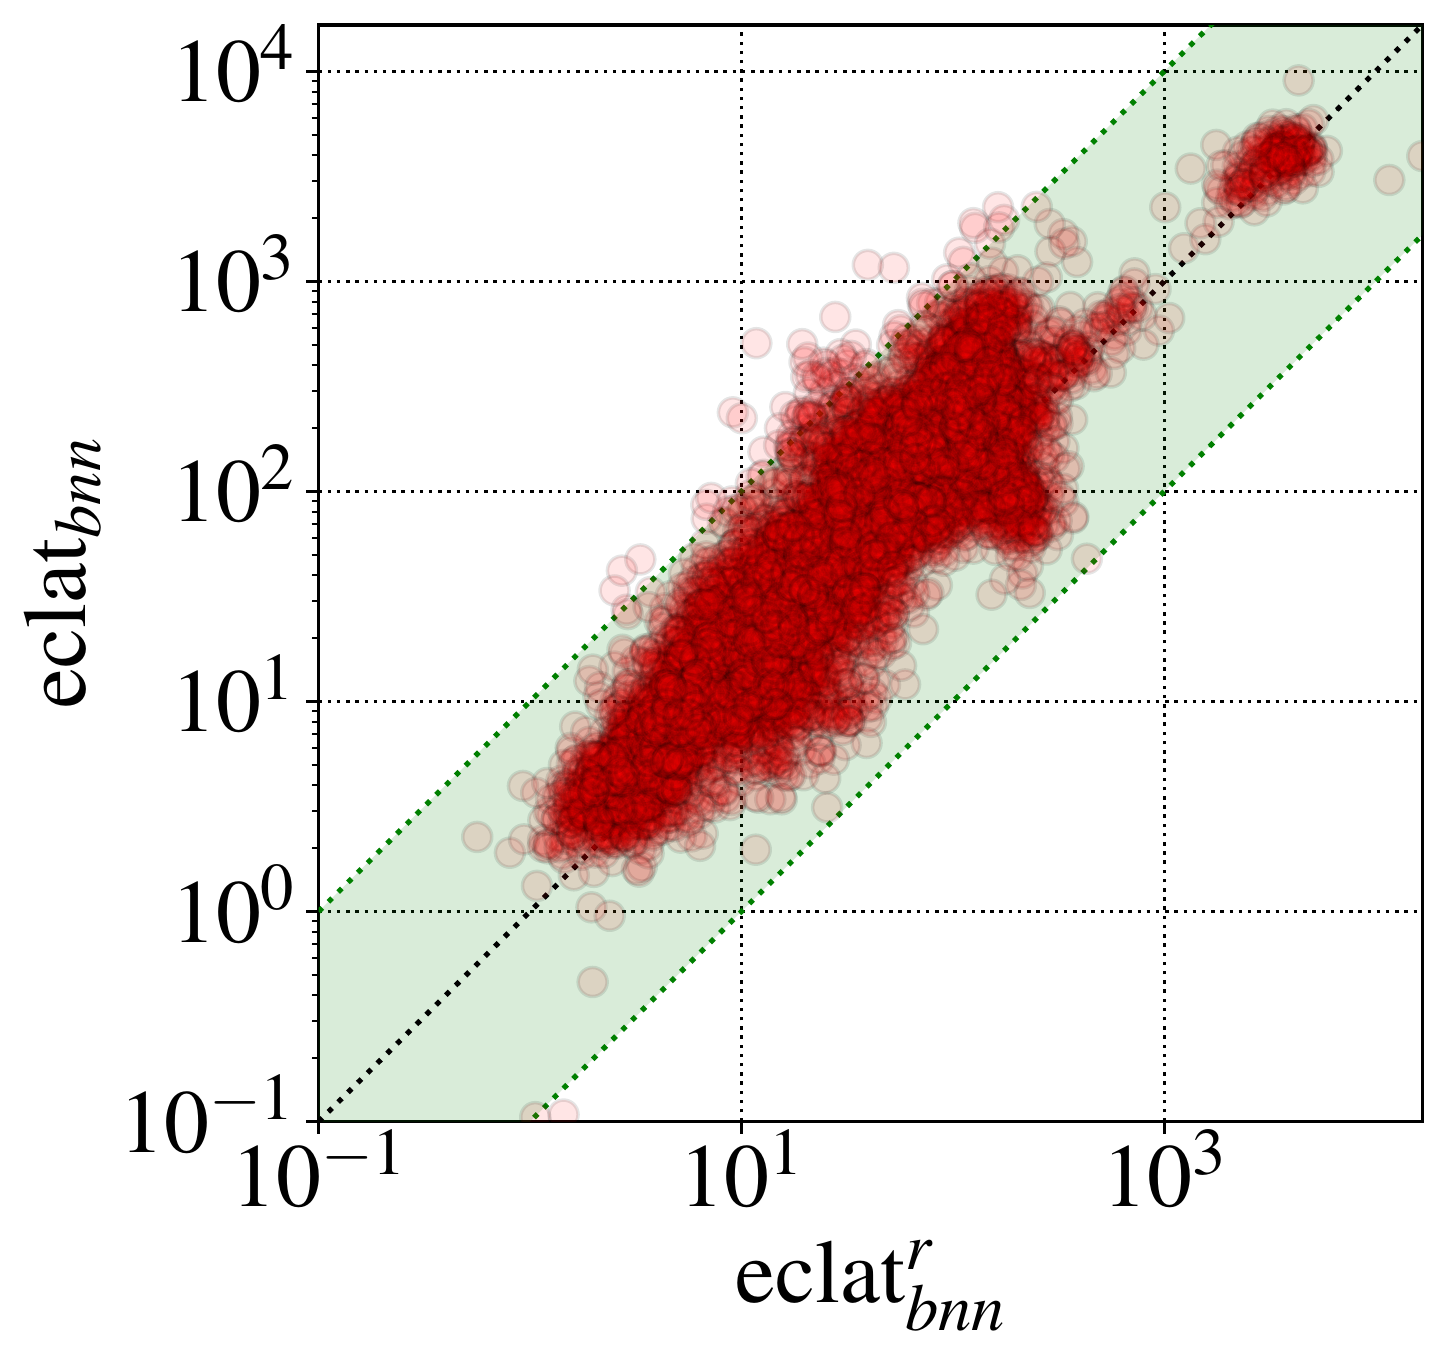}
    \caption{AXp runtime for BNNs}
    \label{fig:abnnaxprtime}
  \end{subfigure}
  \hfill
  \begin{subfigure}[b]{0.236\textwidth}
    \centering
    \includegraphics[width=\textwidth]{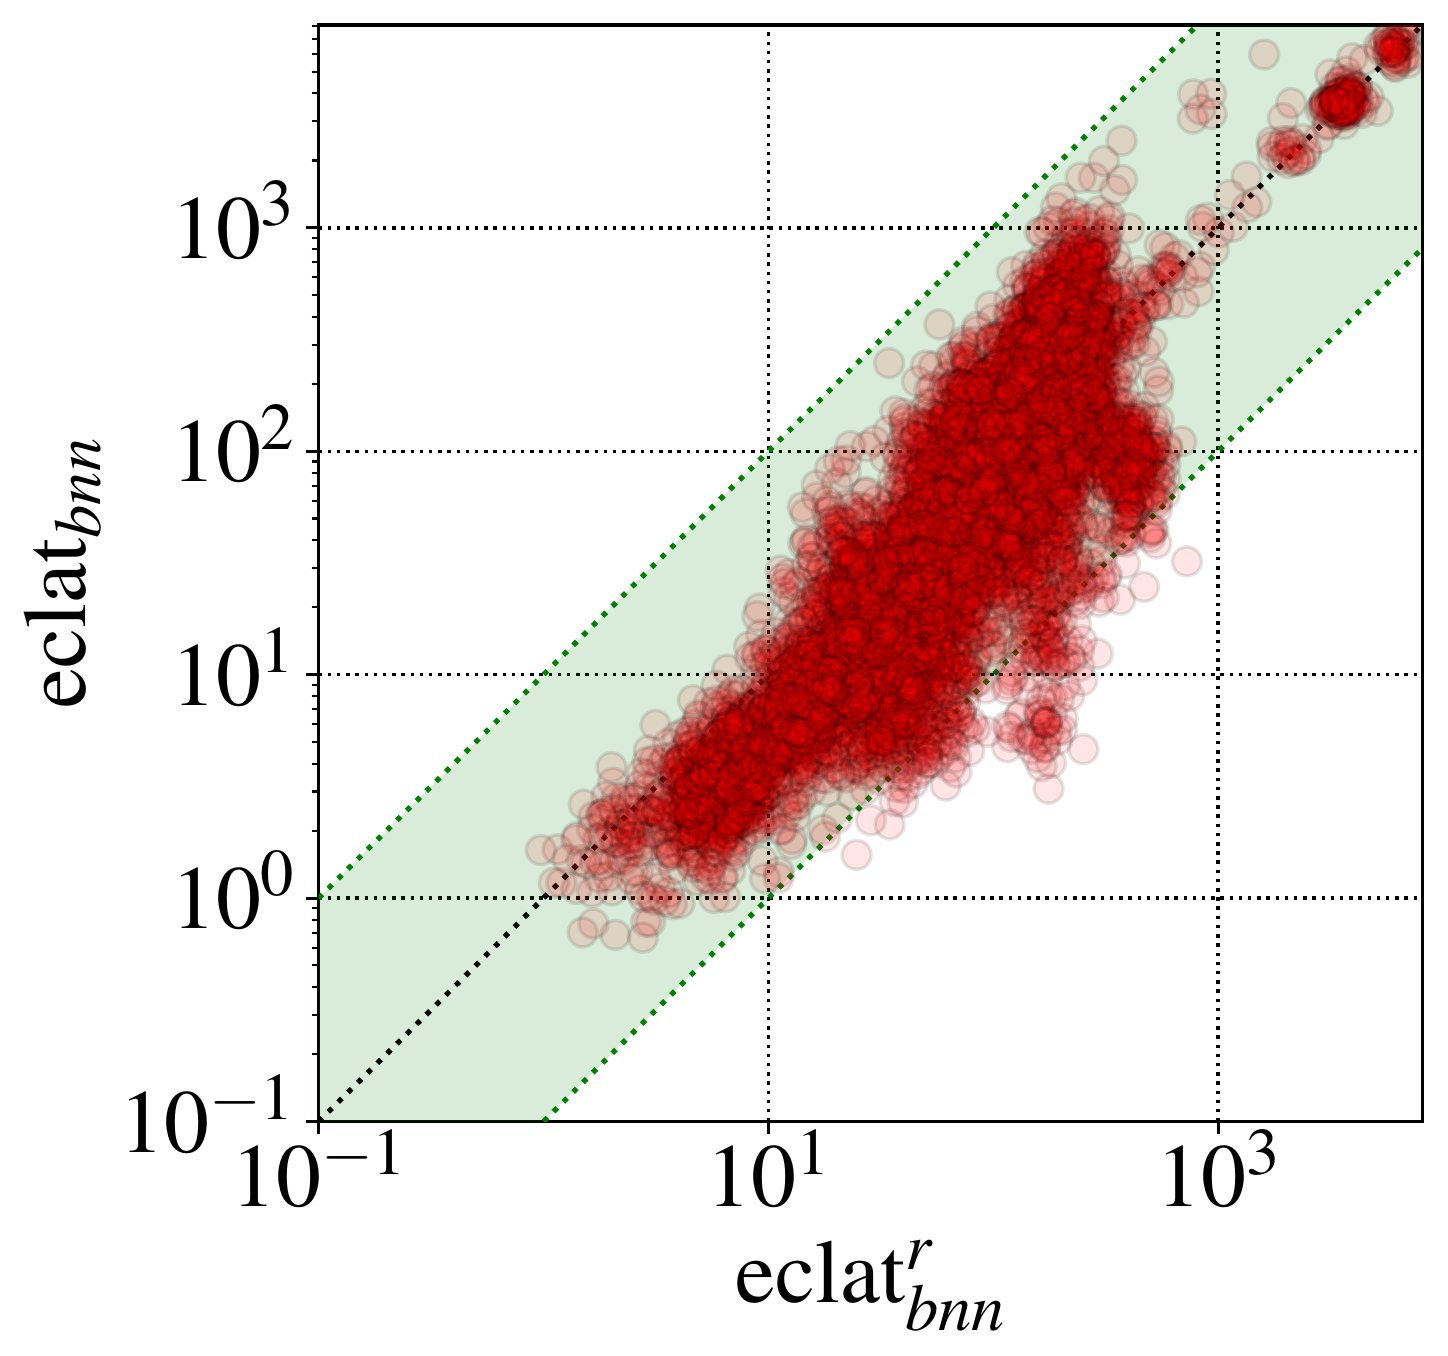}
    \caption{CXp runtime for BNNs}
    \label{fig:abnncxprtime}
  \end{subfigure}
  \hfill
  \begin{subfigure}[b]{0.226\textwidth}
    \centering
    \includegraphics[width=\textwidth]{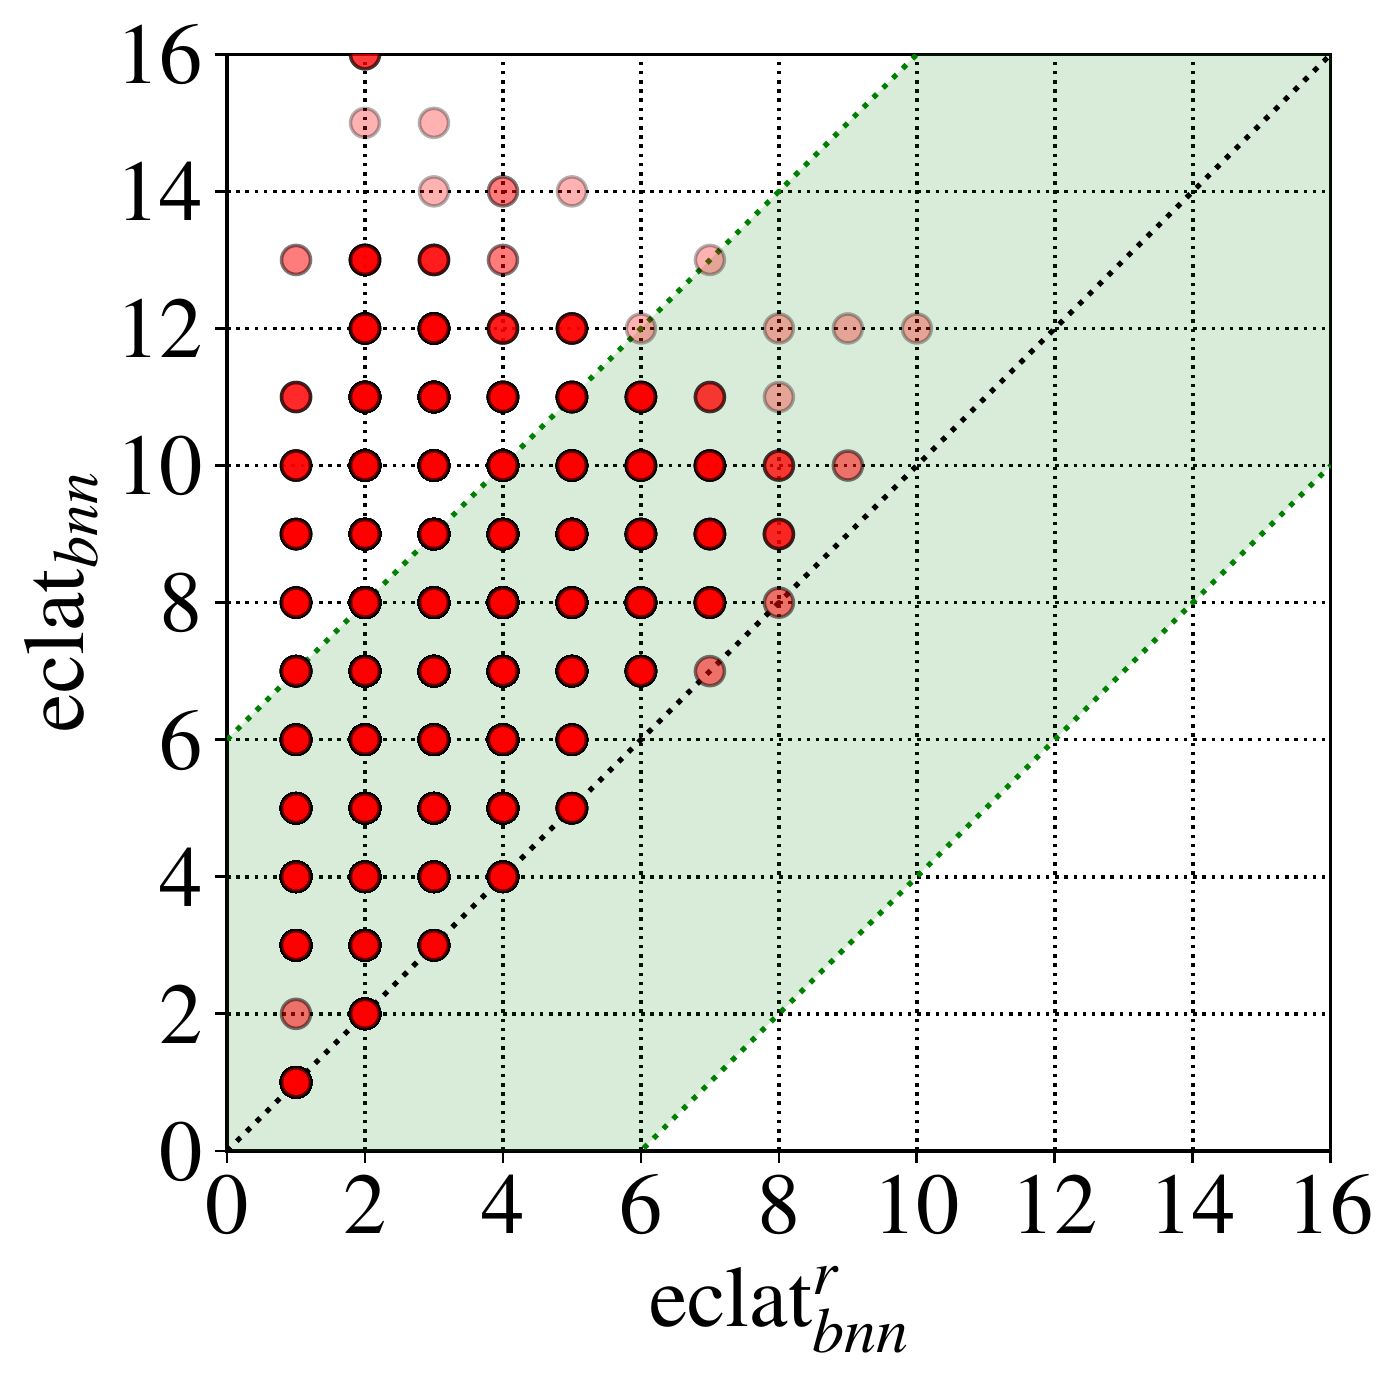}
    \caption{AXp size for BNNs}
    \label{fig:abnnaxp}
  \end{subfigure}%
  \hfill
  \begin{subfigure}[b]{0.226\textwidth}
    \centering
    \includegraphics[width=\textwidth]{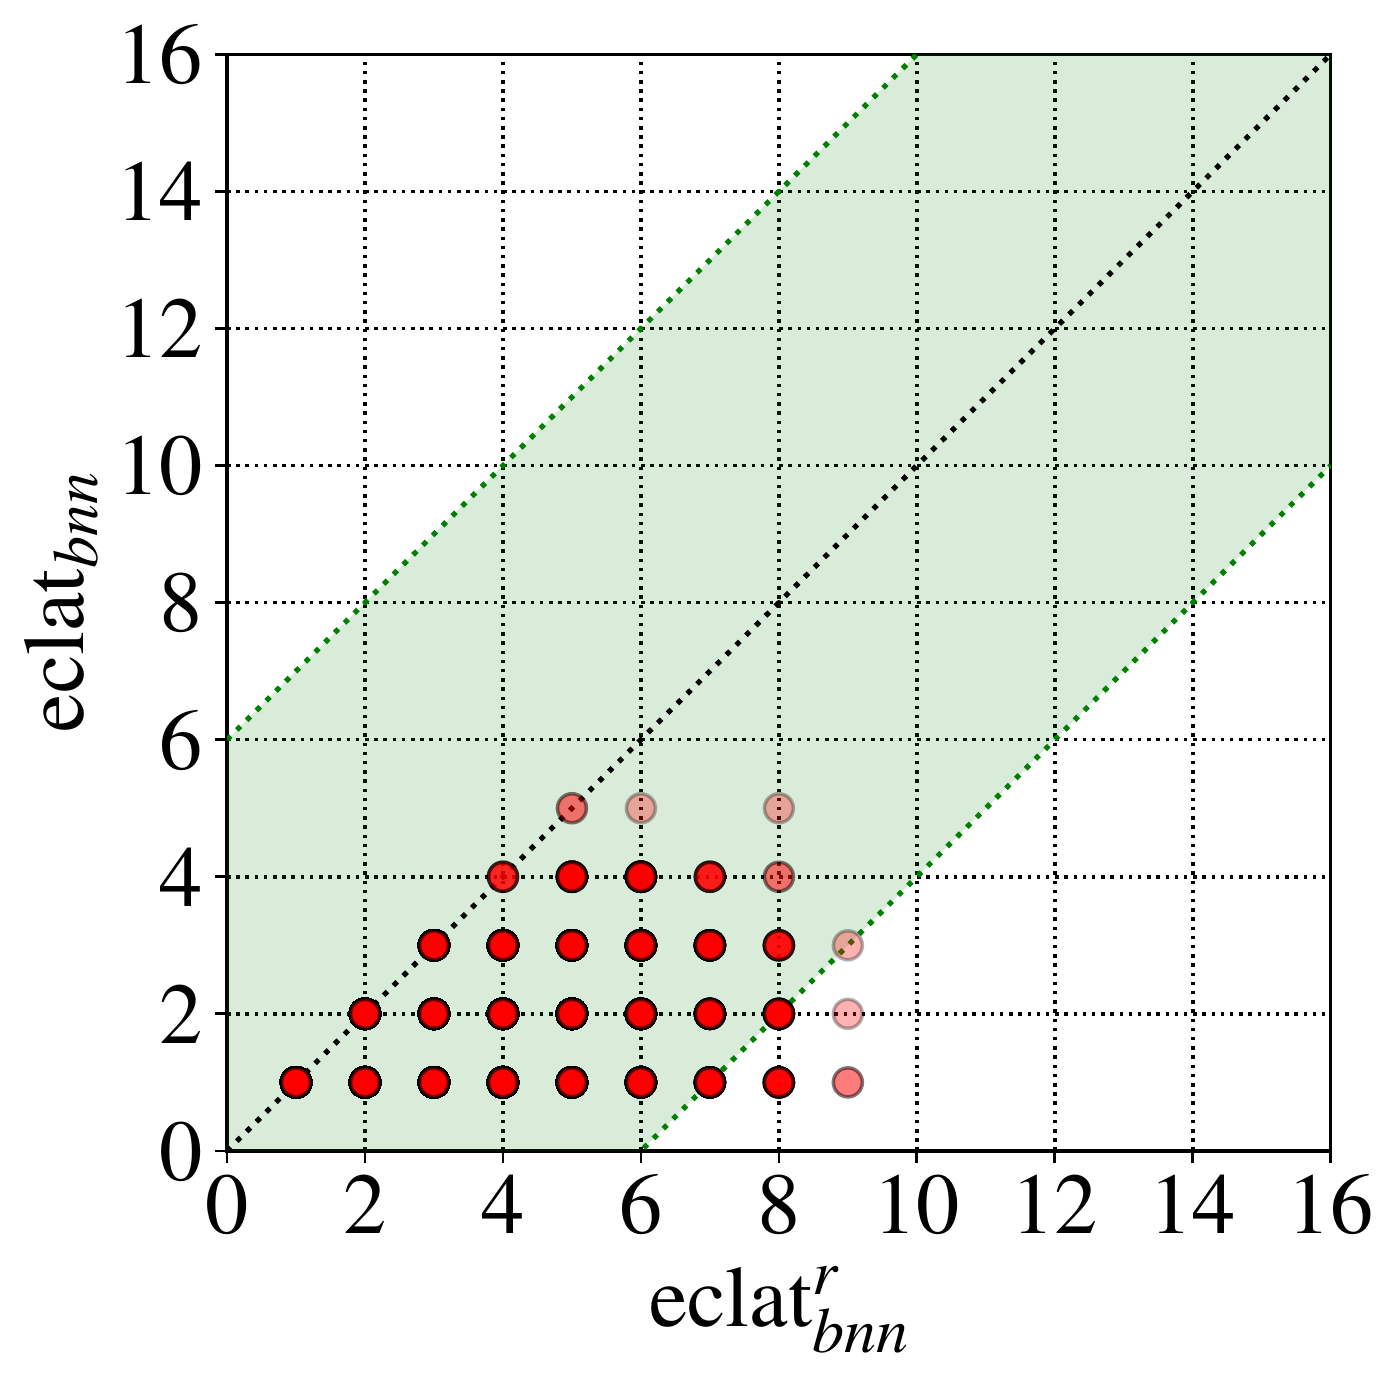}
    \caption{CXp size for BNNs}
    \label{fig:abnncxp}
  \end{subfigure}
    \caption{Runtime~(ms) and explanation size for BNNs w/wo Eclat-assisted background knowledge.}
  \label{fig:abnnxp}
\end{figure*}

\newpage
\section{Eclat-Assisted Explanations}
Figure~\ref{fig:adlxp}, Figure~\ref{fig:abtxp} and Figure~\ref{fig:abnnxp} evaluate
the proposed approach to computing formal explanations for DLs, BTs,
and BNNs, taking into accounting the background knowledge extracted by
Eclat.
Note that only $58$ solved datasets are considered.
Similar to \emph{xcon}$_{\ast}$ discussed in Section~\ref{sec:resexp},
\emph{eclat}$_{\ast} \in \{dl, bt, bnn\}$ indicates the proposed approach
to explain DL, BT, and BNN models
without background knowledge, respectively.
Moreover, \emph{eclat}$^r_{\ast}$ is used to indicate
the configurations applying background knowledge extracted
by Eclat.

\paragraph{Scalability.}

In contrast to the case of the background knowledge extracted by
\emph{xcon}, where the performance of AXp computation for the 3 models
is improved and the performance of CXp computation for BTs as well as
BNNs is not degraded, the use of background knowledge extracted by
Eclat degrades the performance of CXp generation for DLs as well as
both AXp and CXp computation for BTs.
This is because the number of rules extracted by Eclat dramatically
increases compared to \emph{xcon} and taking this larger background
knowledge into account slows down the underlying reasoner.

\paragraph{Explanation Quality.}
Similar observations as for \emph{xcon} can be made, i.e. background
knowledge extracted by Eclat triggers AXp size reduction across the 3
models, while the size of CXps can increase due to the background
knowledge.

\begin{figure*}[h!]
	\centering
	\begin{subfigure}[b]{0.33\textwidth}
    \centering
    \includegraphics[width=\textwidth]{hexp/rtime/cactus_dl_inst_rtime}
    \caption{Runtime for DLs}
    \label{fig:dlhrtime}
  \end{subfigure}
  \hfill
  \begin{subfigure}[b]{0.315\textwidth}
    \centering
    \includegraphics[width=\textwidth]{hexp/rtime/cactus_bt_inst_rtime}
    \caption{Runtime for BTs}
    \label{fig:bthrtime}
  \end{subfigure}
  \hfill
  \begin{subfigure}[b]{0.33\textwidth}
    \centering
    \includegraphics[width=\textwidth]{hexp/rtime/cactus_bnn_inst_rtime}
    \caption{Runtime for BNNs}
    \label{fig:bnnhrtime}
  \end{subfigure}
  \caption{Runtime~(ms) of the considered explainers per explanation for DLs, BTs and BNNs.}
  \label{fig:hrtime}
\end{figure*}

\begin{figure*}[h!]
	\centering
	\begin{subfigure}[b]{0.32\textwidth}
    \centering
    \includegraphics[width=\textwidth]{hexp/size/size_scatter_lime_dl_nobg}
    \caption{Size for DLs without knowledge}
    \label{fig:dllimenobg}
  \end{subfigure}
  \hfill
  \begin{subfigure}[b]{0.33\textwidth}
    \centering
    \includegraphics[width=\textwidth]{hexp/size/size_scatter_lime_bt_nobg}
    \caption{Size for BTs without knowledge}
    \label{fig:btlimenobg}
  \end{subfigure}
  \hfill
  \begin{subfigure}[b]{0.32\textwidth}
    \centering
    \includegraphics[width=\textwidth]{hexp/size/size_scatter_lime_bnn_nobg}
    \caption{Size for BNNs without knowledge}
    \label{fig:bnnlimenobg}
  \end{subfigure}
  \hfill
  \begin{subfigure}[b]{0.32\textwidth}
    \centering
    \includegraphics[width=\textwidth]{hexp/size/size_scatter_lime_dl_bg}
    \caption{Size for DLs with knowledge}
    \label{fig:dllimebg}
  \end{subfigure}
  \hfill
  \begin{subfigure}[b]{0.33\textwidth}
    \centering
    \includegraphics[width=\textwidth]{hexp/size/size_scatter_lime_bt_bg}
    \caption{Size for BTs with knowledge}
    \label{fig:btlimebg}
  \end{subfigure}
  \hfill
  \begin{subfigure}[b]{0.32\textwidth}
    \centering
    \includegraphics[width=\textwidth]{hexp/size/size_scatter_lime_bnn_bg}
    \caption{Size for BNNs with knowledge}
    \label{fig:bnnlimebg}
  \end{subfigure}
  \caption{Explanation size reduction for correct LIME's explanations w/wo background knowledge.}
  \label{fig:limesize}
\end{figure*}

\begin{figure*}[h!]
	\centering
	\begin{subfigure}[b]{0.32\textwidth}
    \centering
    \includegraphics[width=\textwidth]{hexp/size/size_scatter_shap_dl_nobg}
    \caption{Size for DLs without knowledge}
    \label{fig:dlshapnobg}
  \end{subfigure}
  \hfill
  \begin{subfigure}[b]{0.32\textwidth}
    \centering
    \includegraphics[width=\textwidth]{hexp/size/size_scatter_shap_bt_nobg}
    \caption{Size for BTs without knowledge}
    \label{fig:btshapnobg}
  \end{subfigure}
  \hfill
  \begin{subfigure}[b]{0.32\textwidth}
    \centering
    \includegraphics[width=\textwidth]{hexp/size/size_scatter_shap_bnn_nobg}
    \caption{Size for BNNs without knowledge}
    \label{fig:bnnshapnobg}
  \end{subfigure}
  \hfill
  \begin{subfigure}[b]{0.32\textwidth}
    \centering
    \includegraphics[width=\textwidth]{hexp/size/size_scatter_shap_dl_bg}
    \caption{Size for DLs with knowledge}
    \label{fig:dlshapbg}
  \end{subfigure}
  \hfill
  \begin{subfigure}[b]{0.32\textwidth}
    \centering
    \includegraphics[width=\textwidth]{hexp/size/size_scatter_shap_bt_bg}
    \caption{Size for BTs with knowledge}
    \label{fig:btshapbg}
  \end{subfigure}
  \hfill
  \begin{subfigure}[b]{0.32\textwidth}
    \centering
    \includegraphics[width=\textwidth]{hexp/size/size_scatter_shap_bnn_bg}
    \caption{Size for BNNs with knowledge}
    \label{fig:bnnshapbg}
  \end{subfigure}
  \caption{Explanation size reduction for correct SHAP's explanations w/wo background knowledge.}
  \label{fig:shapsize}
\end{figure*}

\begin{figure*}[h!]
	\centering
	\begin{subfigure}[b]{0.32\textwidth}
    \centering
    \includegraphics[width=\textwidth]{hexp/size/size_scatter_anchor_dl_nobg}
    \caption{Size for DLs without knowledge}
    \label{fig:dlanchornobg}
  \end{subfigure}
  \hfill
  \begin{subfigure}[b]{0.33\textwidth}
    \centering
    \includegraphics[width=\textwidth]{hexp/size/size_scatter_anchor_bt_nobg}
    \caption{Size for BTs without knowledge}
    \label{fig:btanchornobg}
  \end{subfigure}
  \hfill
  \begin{subfigure}[b]{0.33\textwidth}
    \centering
    \includegraphics[width=\textwidth]{hexp/size/size_scatter_anchor_bnn_nobg}
    \caption{Size for BNNs without knowledge}
    \label{fig:bnnanchornobg}
  \end{subfigure}
  \hfill
  \begin{subfigure}[b]{0.32\textwidth}
    \centering
    \includegraphics[width=\textwidth]{hexp/size/size_scatter_anchor_dl_bg}
    \caption{Size for DLs with knowledge}
    \label{fig:dlanchorbg}
  \end{subfigure}
  \hfill
  \begin{subfigure}[b]{0.33\textwidth}
    \centering
    \includegraphics[width=\textwidth]{hexp/size/size_scatter_anchor_bt_bg}
    \caption{Size for BTs with knowledge}
    \label{fig:btanchorbg}
  \end{subfigure}
  \hfill
  \begin{subfigure}[b]{0.33\textwidth}
    \centering
    \includegraphics[width=\textwidth]{hexp/size/size_scatter_anchor_bnn_bg}
    \caption{Size for BNNs with knowledge}
    \label{fig:bnnanchorbg}
  \end{subfigure}
  \caption{Explanation size reduction for correct Anchor's explanations w/wo background knowledge.}
  \label{fig:anchorsize}
\end{figure*}

\newpage \section{Detailed Experimental Results for LIME, SHAP, and
Anchor}\label{ares:hres} This appendix estimates the efficiency and
explanation quality of the 3 heuristic approaches, i.e. LIME, SHAP,
and Anchor.
In particular, we assess the runtime of explanation computation as
well as check how the size of correct heuristic explanations can be
reduced with and without background knowledge provided.

\paragraph{Scalability.}
Figure~\ref{fig:hrtime} details the runtime of a single explanation
generation for a data instance among LIME, SHAP, Anchor, \emph{xcon},
and \emph{xcon}$^r$.
Hereinafter, \emph{lime}$_{\ast}$, \emph{shap}$_{\ast}$, and
\emph{anchor}$_{\ast}$, s.t.\ $\ast\in\{dl, bt, bnn\}$, indicate LIME,
SHAP, and Anchor, respectively, applied to computing explanations for
DLs, BTs, and BNNs, while \emph{xcon}$^r_{\ast, xp}$ and
\emph{xcon}$_{\ast, xp}$  represent the proposed approach to computing
AXps or CXps for the three models with/without background knowledge,
s.t.\ $\ast\in\{dl, bt, bnn\}$ and $xp\in\{axp, cxp\}$.
Here, the setup described in~Section~\ref{sec:resexp} is used for
\emph{xcon} as well as \emph{xcon}$^r$, and the runtime of computing a
single formal explanation (either AXp or a CXp) is considered.
Figure~\ref{fig:hrtime} demonstrates that both \emph{xcon} and
\emph{xcon}$^r$ outperform LIME and Anchor for all the 3 models, where
each explanation is computed in less than 1 second.
LIME and Anchor achieve similar performance for DL and BNN models,
while LIME outweighs Anchor when generating explanations for BTs.
However, the worst performance for DL and BNN models is demonstrated
by SHAP while, surprisingly, SHAP outperforms the other competitors
for BTs models.

\ignore{
}

\paragraph{Explanation Quality.}
Although explanation correctness dramatically increases when
background knowledge is applied, the lack of explanation minimality
guarantees is troublesome, as the large size of \emph{correct}
heuristic explanations can render such explanations uninterpretable.
Here, we evaluate the size of correct explanations computed by LIME,
SHAP, and Anchor.
In particular, for each heuristic explanation computed either by LIME,
SHAP, or Anchor for any of the three models considered, we extract a
subset-minimal AXp from it and compare the size of the original
heuristic explanation against the size of the result AXp.
The comparisons are illustrated in Figure~\ref{fig:limesize},
\ref{fig:shapsize}, and \ref{fig:anchorsize}.
As can be observed, a lion's share of correct explanations computed by
LIME, SHAP, and Anchor are far from being minimal, and the size
reduction obtained when extracting a subset-minimal AXp is provided.
Unsurprisingly and confirming the results discussed in the paper, the
use of background knowledge enables us to achieve a higher rate of
explanation size reduction.
